# Supplementary material for: The build-up of the cD halo of M87 - evidence for accretion in the last Gyr
Source: arXiv:1504.04369 source file (2015-06-08)
Supplement: Supplementary file 1 [file appendix.tex]

\onecolumn{ \begin{appendix} 
\section{Gaussian Mixture models}
The Gaussian Mixture Models (GMM) is a probabilistic model which
assumes that a distribution of points is drawn from a mixture of
finite number of Gaussian distribution with unknown parameters. The
GMM results then in a linear combination of $K$ Gaussian probability
density functions (pdfs), or components, expressed by:

\begin{equation}
p({\bf x})=\sum_{k=1}^{K} p({\bf x}|k)P(k),
\end{equation} 
\label{sec3}
where $P(k)$ is the mixture weight that satisfies the conditions $0
\le P(k) \le 1$ and $\sum_{k=1}^{K}P(k)$=1; and $ p({\bf x}|k)$ is the
height of the $k$th component pdf at vector ${\bf x}$.

The GMM classifier implemets the Expectation-Maximization (EM)
algorithm for fitting a mixture of Gaussian pdfs, that can be
summarised in 4 main steps:
\begin{enumerate}
\item Given a sample $X$ of $x_{n}$ data points, we give an initial
  set of $K=3$ gaussian component pdfs and their weights, i.e. we
  assign initial estimates of mean values, $\mu_{k}$,
  dispersions, $\sigma_{k}$ and relative importance of each components,
  $P(k)$, with $k=1,...,K$.
\item \textbf{E-step}. We then determine the \textit{responsibility} $P(k|x_{n})$ of each component pdfs for each data point $ x_{n}$ as:
\begin{equation}
p_{kn}\equiv P(k| x_{n})=\frac{p( x_{n}|k)P(k)}{p( x_{n})},
\end{equation}
with GMM likelihood $p( x_{n})= \sum_{k=1}^K p( x_{n}|k)P(k)$.

\item \textbf{M-step}. The component pdfs are re-estimated based on the data and the responsibilities as:

\begin{equation}
P(k)=\frac{1}{N} \sum_{n=1}^{N}p_{kn}
\end{equation}
\begin{equation}
\mu_{k}=\frac{\sum_{n}p_{kn}x_{n}}{\sum_{n}p_{kn}}
\end{equation}
\begin{equation}
\sigma^{2}_{k}=\frac{\sum_{n}p_{kn}(x_{n}-\mu_{k})^2}{\sum_{n}p_{kn}}.
\end{equation}

\item Steps 2. and 3. are repeted till the GMM likelihood
  $p(X)=\prod_{n=1}^{N}p(x_{n})$ of the entire dataset does not change
  aprreciabily.
\end{enumerate}

The EM algorithm is an iterative process that assignes to each point of
the distribution the class of the Gaussian it mostly
probabibly belongs to.

\end{appendix}}
